# Supplementary material for: AeroTraj: Trajectory Planning for Fast, and Accurate 3D Reconstruction Using a Drone-based LiDAR
Source: arXiv:2104.08634 source file (2024-06-26)
Supplement: Supplementary file 1 [file appendix.tex]

\setcounter{section}{0}
\setcounter{algocf}{0}
\setcounter{figure}{0}
\setcounter{table}{0}

\section{Appendix}
\label{s:appendix}

\subsection{Recon Flight}
\label{s:app_recon_flight}
The goal of the recon flight is to survey the area and find the boundary of the structure as fast as possible. \sysname uses a flight trajectory as shown in \figref{fig:recon_traj} in which parallel scans of length $d$ are separated by a scan width $s$. In designing the recon flight, \sysname can change the height, speed and LiDAR orientation of the drone. To find the right set of parameters, we performed an exhaustive parameter sweep. 

\parab{Optimum height for recon.} To find the optimum height for the recon flight, we planned recon trajectories for a 20~m building (within a 300~m x 300~m area) in AirSim at different heights (from 40~m to 90~m). We flew the drone and ran the boundary estimation on the collected \textit{highly compressed} LiDAR point clouds at 10~Hz. For each height, we collected data and ran the boundary detection module five times. Higher flights increase scan width (~\figref{fig:lidar_coverage_area}) at the expense of point density. However, \sysname's boundary detection algorithm is robust to lower density point clouds (up till 80~m) and can accurately estimate the boundary of the building from a height of upto 80~m. \figref{fig:recon_height} shows the 2D boundary detection accuracy, completeness (lower is good) and flight duration (as a proxy for battery usage) as a function of the height of the drone. We find that at 80~m (or 60~m from the building), \sysname can jointly optimize for battery efficiency and boundary detection accuracy. At 80~m, \sysname can complete the recon flight in 150~seconds and estimate the boundary to within 2.5~m accuracy and completeness. Beyond 80~m, the scan width and point density decrease. This results in longer flights and higher boundary detection accuracy and completeness.

% \begin{figure}[t]
%   \centering
%   \includegraphics[width=0.5\columnwidth]{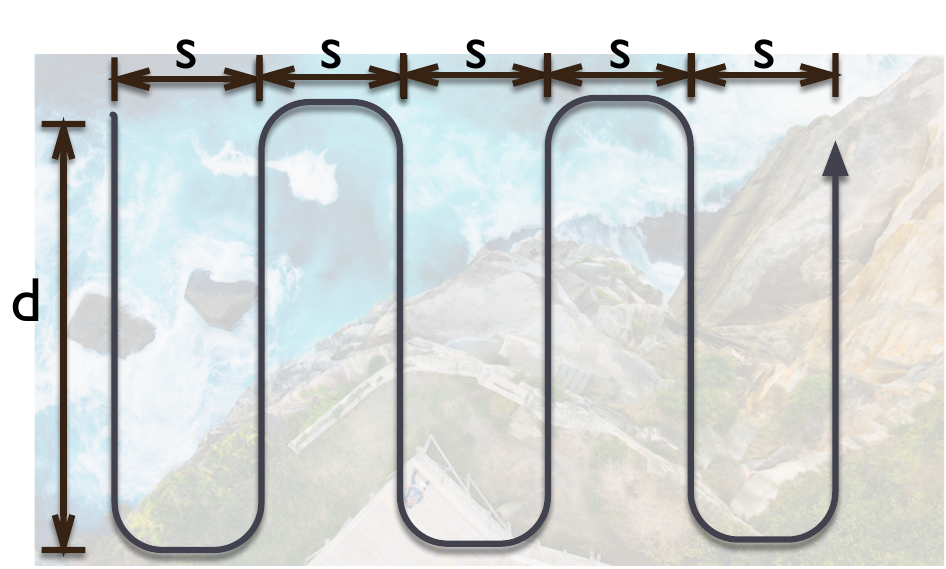}
%   \caption{Recon flight trajectory for \sysname.}
%   \label{fig:recon_traj}
% \end{figure}

% \begin{figure}[t]
%   \centering
%   \includegraphics[width=0.5\columnwidth]{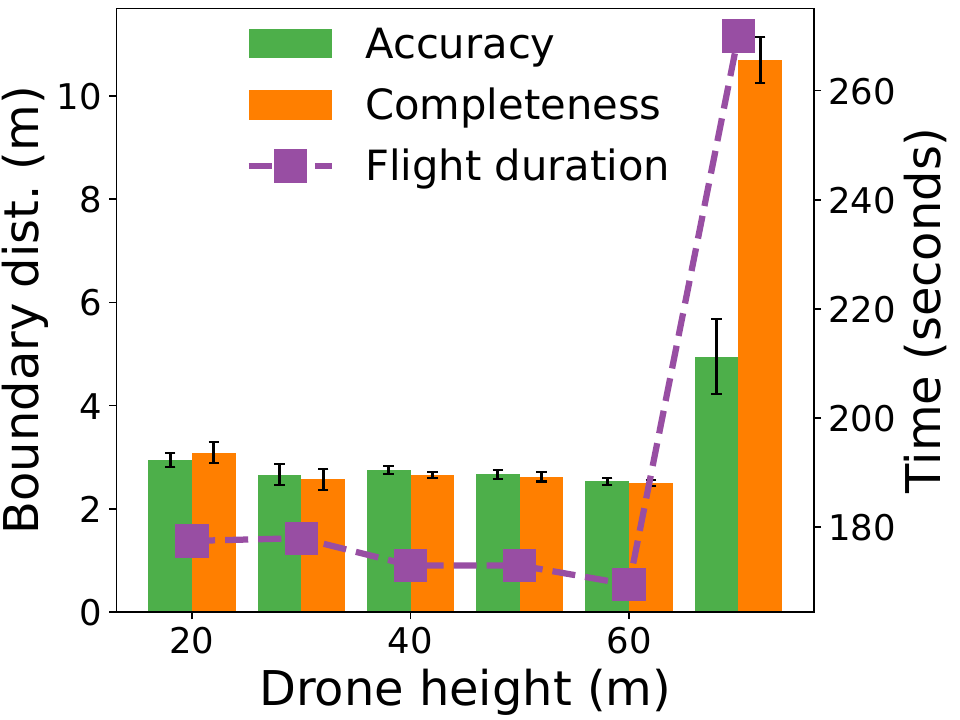}
%   \caption{Finding the right height for boundary detection accuracy and battery efficiency in the recon flight.}
%   \label{fig:recon_height}
% \end{figure}

\parab{Optimum speed for recon.}
To find the optimum speed for the recon flight, we planned a recon trajectory for the drone to fly over the same 20~m building at a height of 80~m from the ground. We flew the drone in the planned trajectory at speeds from 1~m/s to 8~m/s and ran boundary detection on the \textit{highly compressed} point clouds at 10~Hz. For each speed, we collected data and ran the boundary detection module five times. \figref{fig:recon_speed} illustrates the effect of drone speed on the boundary detection accuracy, completeness and the flight duration. A higher speed results in lower flight duration but at the expense of boundary detection accuracy and completeness. Even then, \sysname robustly extracts the boundary up till 6~m/s. At higher speeds, the overlap between consecutive frames is smaller and hence \sysname cannot accurately stitch the frames together. As such, \sysname flies the drone at the sweet spot \ie 4~m/s where the flight duration is approximately 150~seconds and accuracy and completeness are 2.5~m.
% the scan width and hence the total flight time decreases (\figref{ Although a drone flight at a higher altitude can increase ground coverage, yielding better battery efficiency, it comes at the expense of lower point density. However, \sysname's boundary detection algorithm is robust to   A recon flight at a high altitude (upto a certain limit) can reduce 

\parab{Optimum LiDAR orientation.}
LiDAR orientation controls scan width and point cloud overlap. A parallel orientation means larger overlap but small scan width $s$. On the other hand, a perpendicular orientation means smaller overlap but larger scan width $s$. Larger scan width $s$ means a smaller flight duration (\figref{fig:recon_traj}). A large overlap means better scan matching accuracy. Since \sysname uses GPS for stitching in the recon phase, so it is robust to the overlap. Hence, to minimize flight duration, it uses a perpendicular orientation of the LiDAR. We conducted experiments (omitted for brevity) without different orientations of the LiDAR and confirmed that a perpendicular orientation minimzes flight duration without any loss in accuracy/completeness.
% We omit a detailed discussion, but summarize two results. First, recon flights can be short, because boundary detection is less sensitive to point density and overlap. So, it can use perpendicular orientation, fly at 60~m from the building at 4~m/s. Second, boundary detection can tolerate point cloud sub-sampling. \sysname already uses only every other frame, but our evaluations show that boundary detection works well even when using one point cloud every 12 seconds.

% \begin{figure}[b]
%   \centering
%   \includegraphics[width=0.5\columnwidth]{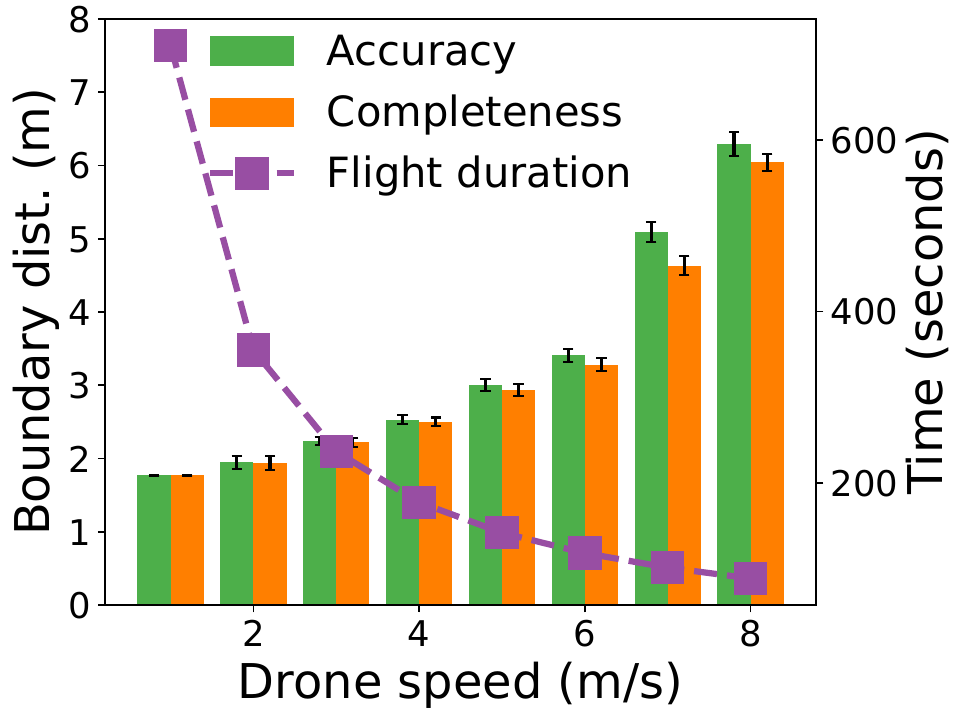}
%   \caption{Finding the right speed for boundary detection accuracy and battery efficiency in the recon flight.}
%   \label{fig:recon_speed}
% \end{figure}

\parab{Boundary extraction for different buildings.}
To show that \sysname can accurately extract the 2D boundary of any building, we collected LiDAR traces of a drone flying over five different buildings in Airsim at a height of 80~m and speed of 4~m/s. We collected data over each building five times. Then, we ran boundary detection on the \textit{highly compressed} point clouds at 10~Hz. We summarize the boundary detection accuracy, completeness and the flight duration in \tabref{tab:recon_buildings}. As expected, the flight duration for all buildings is independent of the underlying building. For all building types, \sysname can accurately extract the boundary of all buildings within 2.5~m accuracy and completeness. This shows that \sysname's boundary detection is scalable to all building shapes.

\begin{table}[t]
\footnotesize
\centering
\begin{tabular}{|c|c|c|c|}
\hline
\begin{tabular}[c]{@{}c@{}}Structure\\ type\end{tabular} & 
\begin{tabular}[c]{@{}c@{}}Flight \\ duration (s)\end{tabular} & 
\begin{tabular}[c]{@{}c@{}}Accuracy\\ (m)\end{tabular} & 
\begin{tabular}[c]{@{}c@{}}Comp.\\ (m)\end{tabular} \\ \hline
Star-shaped        & 150 & 1.39 & 1.67 \\ \hline
H-shaped           & 150 & 1.31 & 1.83 \\ \hline
Plus-shaped        & 150 & 1.35 & 1.55 \\ \hline
Pentagon           & 150 & 2.58 & 2.58 \\ \hline
Rectangular        & 150 & 2.50 & 2.53 \\ \hline
\end{tabular}
\caption{\system boundary estimation accuracy, completeness and flight duration for different building types using high compression.}
% \end{tabular}
\label{tab:recon_buildings}
\end{table}

\parab{Effect of point cloud compression.}
To evaluate the effect of point cloud compression on boundary extraction, we compressed a real-world over the 70~m~x~40~m~x~20~m building with the four different compression profiles described above. Then, we ran our boundary extraction algorithm on the compressed traces. \tabref{tab:recon_compression} shows that \sysname's boundary extraction algorithm is robust to compression. While bringing down bandwidth by a factor of 377, for high compression, \sysname only trades off 36~cm in accuracy and 24~cm in completeness. With higher bandwidths promised with the emergence of 5G, \sysname can achieve the same boundary extraction accuracy as an uncompressed trace.

\begin{table}[t]
\footnotesize
\centering
\begin{tabular}{|c|c|c|c|}
\hline
\begin{tabular}[c]{@{}c@{}}Compression\\ profile\end{tabular} & 
\begin{tabular}[c]{@{}c@{}}Required \\ bandwidth (Mbps)\end{tabular} & 
\begin{tabular}[c]{@{}c@{}}Accuracy\\ (m)\end{tabular} & 
\begin{tabular}[c]{@{}c@{}}Comp.\\ (m)\end{tabular} \\ \hline
Uncompressed        & 480.0 & 1.09 & 1.09 \\ \hline
View-point          & 42.7 & 1.09 & 1.09 \\ \hline
Lossless            & 7.86 & 1.09 & 1.09 \\ \hline
Low                 & 3.80 & 1.09 & 1.10 \\ \hline
Medium              & 2.50 & 1.13 & 1.07 \\ \hline
High                & 1.27 & 1.45 & 1.33 \\ \hline
\end{tabular}
\caption{\system boundary estimation accuracy and completeness for different levels of compression.}
% \end{tabular}
\label{tab:recon_compression}
\end{table}

\parab{Effect of sub-sampling.}
\sysname's boundary detection algorithm runs at 10~fps. A Ouster-64 beam LiDAR generates 20 point clouds per second. So, the boundary detection algorithm must be robust to sub-sampling of point clouds. Our evaluations show that, for a drone traveling at 4~m/s, it works well even when using one point cloud every 3 seconds. Because \sysname's boundary detection uses GPS for stitching, it does not need overlap between 3D frames.

\subsection{Data Collection}
\label{s:app_data_coll}
In this section, we perform a parameter sensitivity study to find the optimum parameters for running SLAM accurately on \textit{real-world} UAV flights. To do this, we report positioning error generated by SLAM. For the lack of accurate ground truth in the real-world, we compare SLAM positions against a GPS trace. Positioning accuracy is directly related to 3D model RMSE because these poses are used to position 3D point cloud in generating a 3D model. A higher positioning error leads to a higher reconstruction error and vice-versa.

\parab{Effect of drone speed.}
Because GPS is erroneous, we only draw qualitative conclusions. As \tabref{tab:real_speed_vs_rmse}, taken from our drone traces, shows, slower flights have lower SLAM error than faster one, and parallel orientations have lower SLAM error than perpendicular. 

\parab{Effect of drone height.}
Similarly, SLAM error increases with height and, in real-world traces, the parallel orientation seems to be significantly better than the perpendicular orientation (\tabref{tab:real_height_vs_rmse}). At a distance of 20~m from the surface of the building, the parallel orientation has the minimum positioning error \ie 1.25~m. Beyond 20~m for parallel and 40~m for perpendicular, SLAM loses track completely because of lower point density.
